# Supplementary material for: Tokenize Image Patches: Global Context Fusion for Effective Haze Removal in Large Images
Source: arXiv:2504.09621 source file (2025-04-13)
Supplement: Supplementary file 1 [file X_suppl.tex]

\clearpage
\setcounter{page}{1}
\maketitlesupplementary

\section{More Details of Experiments}
\vspace{-1mm}
In our experiments, we utilize 3 datasets: \emph{8KDehaze}, \emph{4KID}, and \emph{O-HAZE}. The \emph{4KID} dataset includes 3 subsets: Daytime, Night, and Realtime. For consistency with the other datasets, we select the Daytime subset for training and testing. Since both the \emph{4KID} and \emph{O-HAZE} datasets do not provide pre-split training and test sets, we randomly select 500 samples from the \emph{4KID} dataset and 5 samples from the O-HAZE dataset as the test set. The remaining images from these datasets are used for training. To further enhance the generalization capability of the model, we apply random rotations to the input images during training, ensuring greater variability and robustness in the model's performance.

\vspace{-1mm}
\section{More Details of the \emph{8KDehaze} dataset}
\vspace{-1mm}
To the best of our knowledge, the proposed \emph{8KDehaze} dataset is the first ultra-high-resolution dataset in the field of image dehazing. It consists of 9,000 training pairs and 1,000 test pairs, each with a resolution of 8192 $\times$ 8192 pixels. This dataset offers a valuable resource for advancing large image inference in the dehazing domain. In this section, we provide a detailed description of the dataset’s key features and discuss its potential impact on the development of dehazing algorithms.

\begin{figure*}
    \centering
    \includegraphics[width=\linewidth]{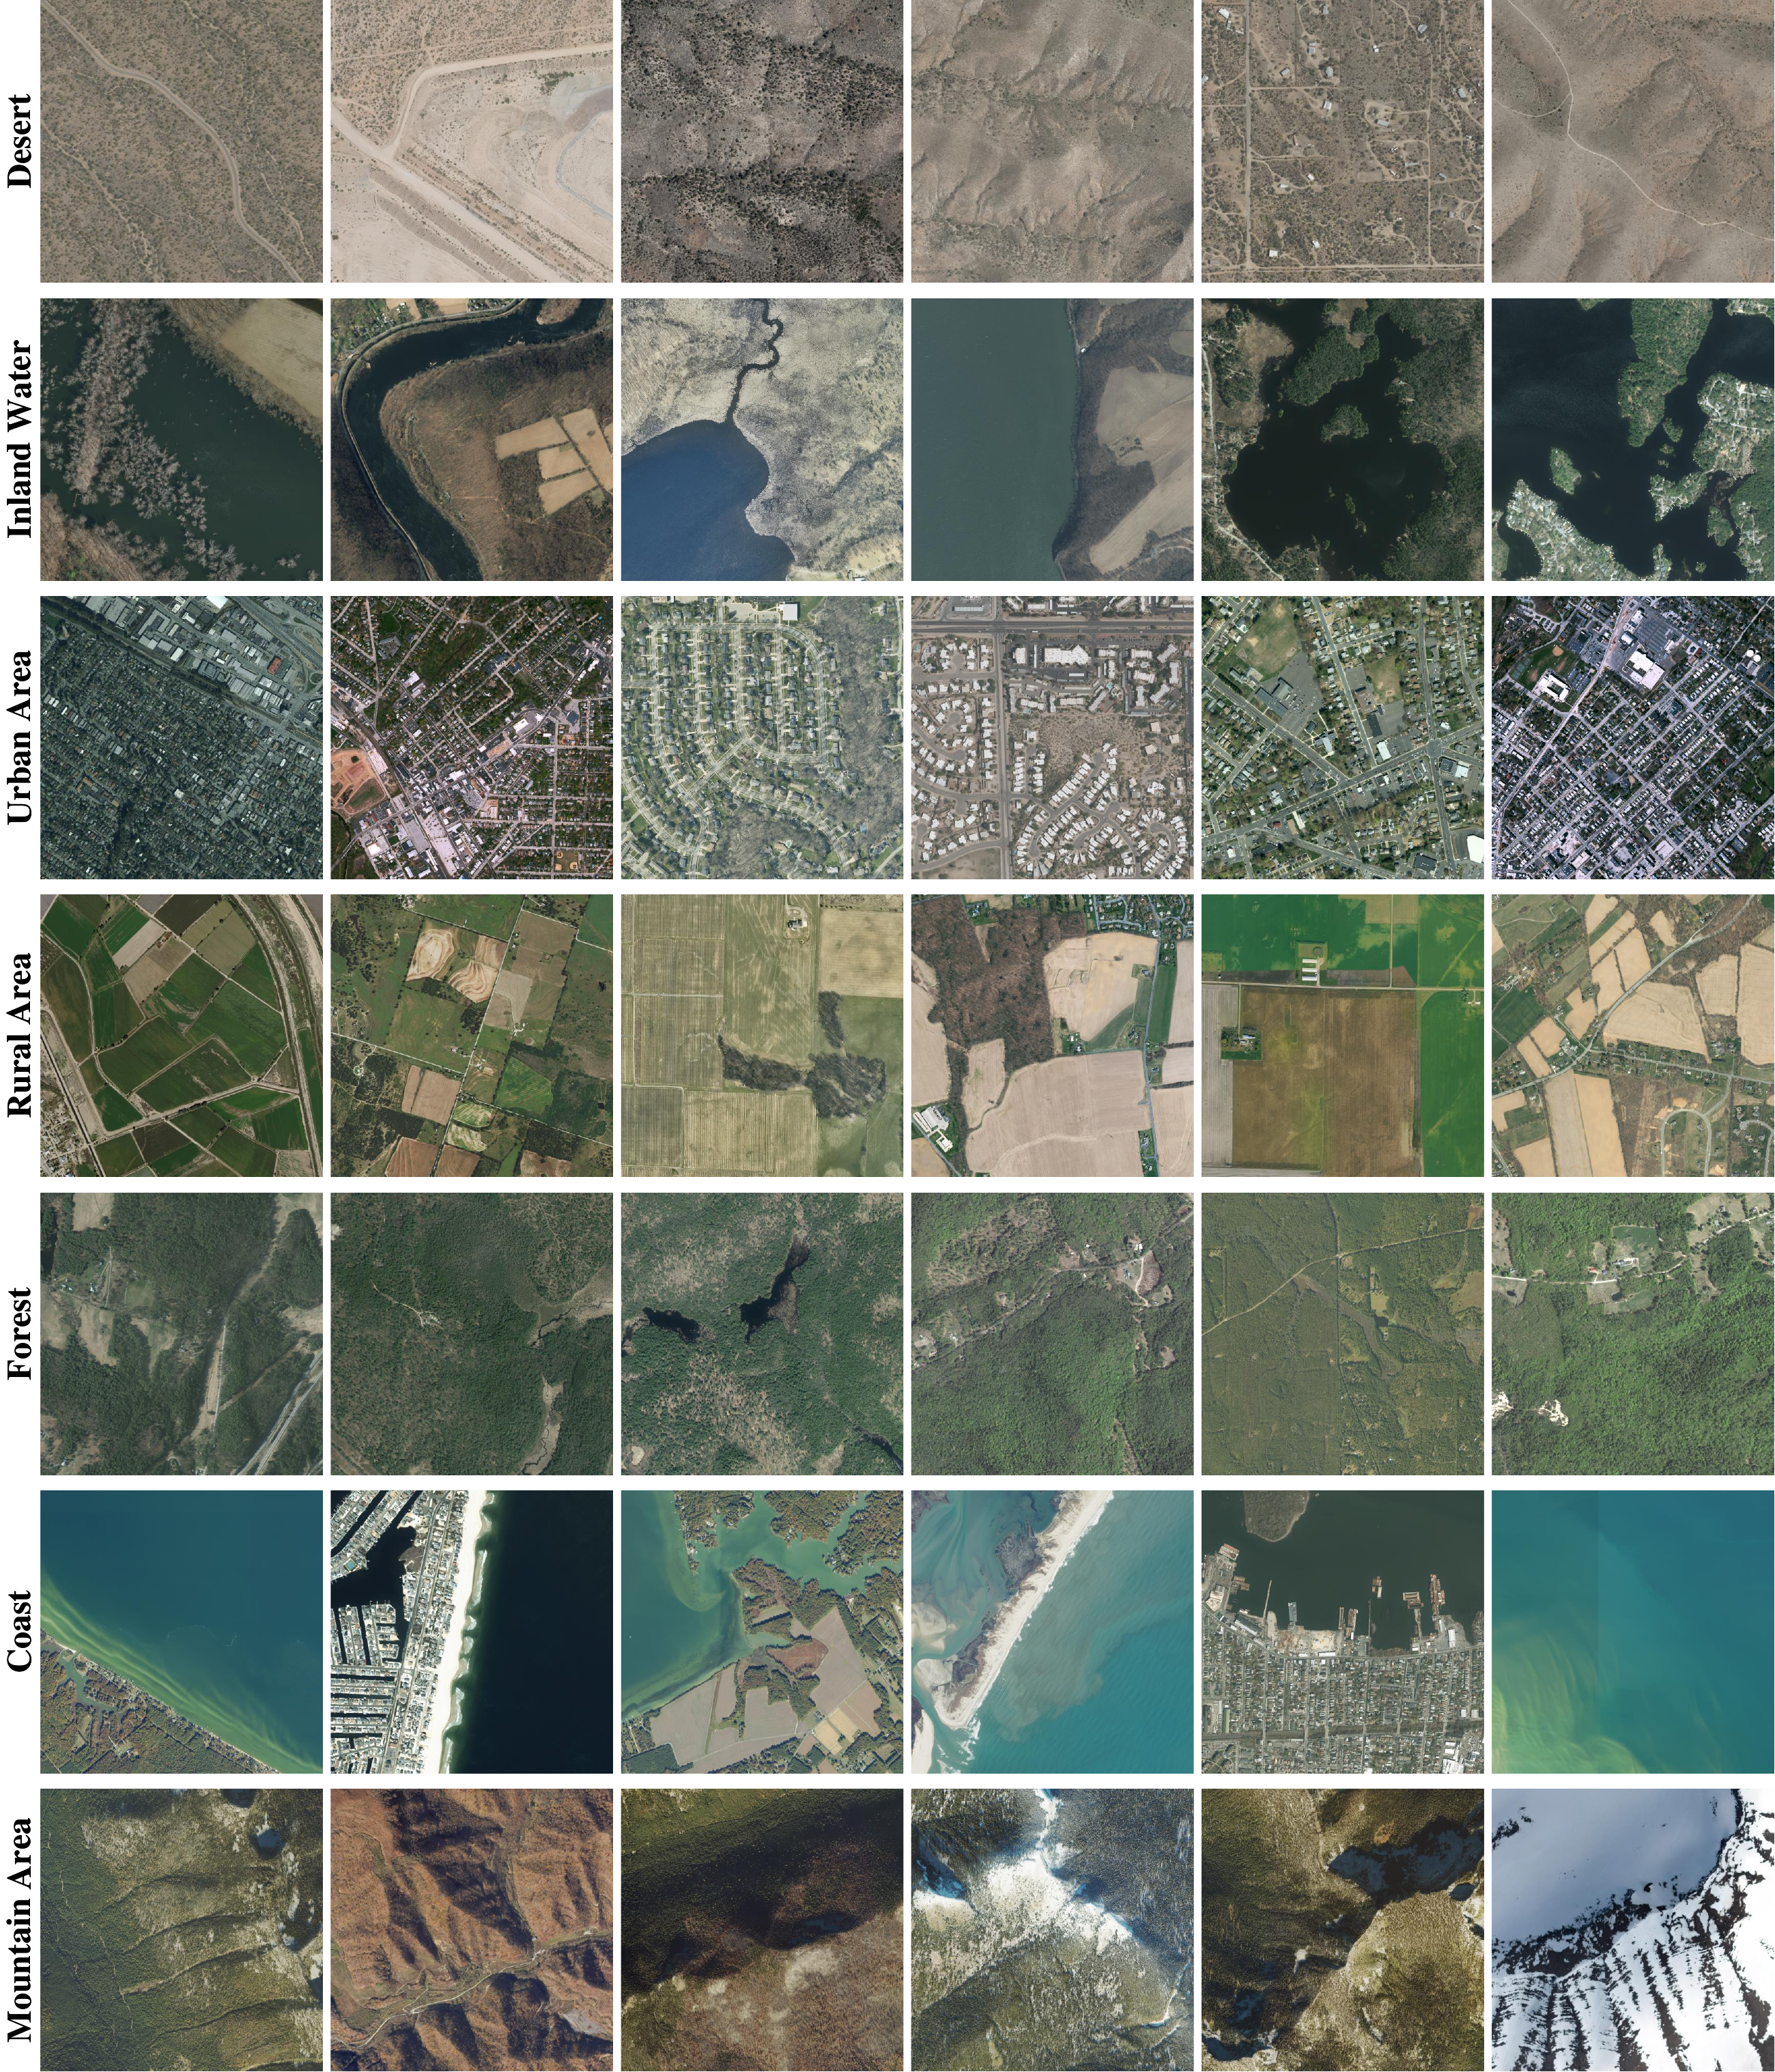}
    \caption{Geographic Diversity of the \emph{8KDehaze} Dataset. The samples in the \emph{8KDehaze} dataset cover seven distinct terrain types: desert, inland waters, urban areas, rural areas, forest, coast, and mountain areas.}
    \label{fig:geo}
\end{figure*}

\vspace{0.3\baselineskip}
\noindent\textbf{Geographical Diversity.} The \emph{8KDehaze} dataset encompasses a wide range of geographical environments, ensuring a comprehensive representation of real-world scenarios. As shown in Figure \ref{fig:geo}, the images are sourced from diverse regions, including desert, inland waters, urban areas, rural landscapes, forest, coastlines, and mountainous terrains. This geographical diversity enables the dataset to capture the various ways in which haze manifests across different topographies and ecosystems. The distribution of images across these categories is uniform, ensuring that models trained on the \emph{8KDehaze} dataset can generalize well to different types of scenes in practical applications.

\begin{figure*}
    \setlength{\belowcaptionskip}{-5pt}
    \centering
    \includegraphics[width=\linewidth]{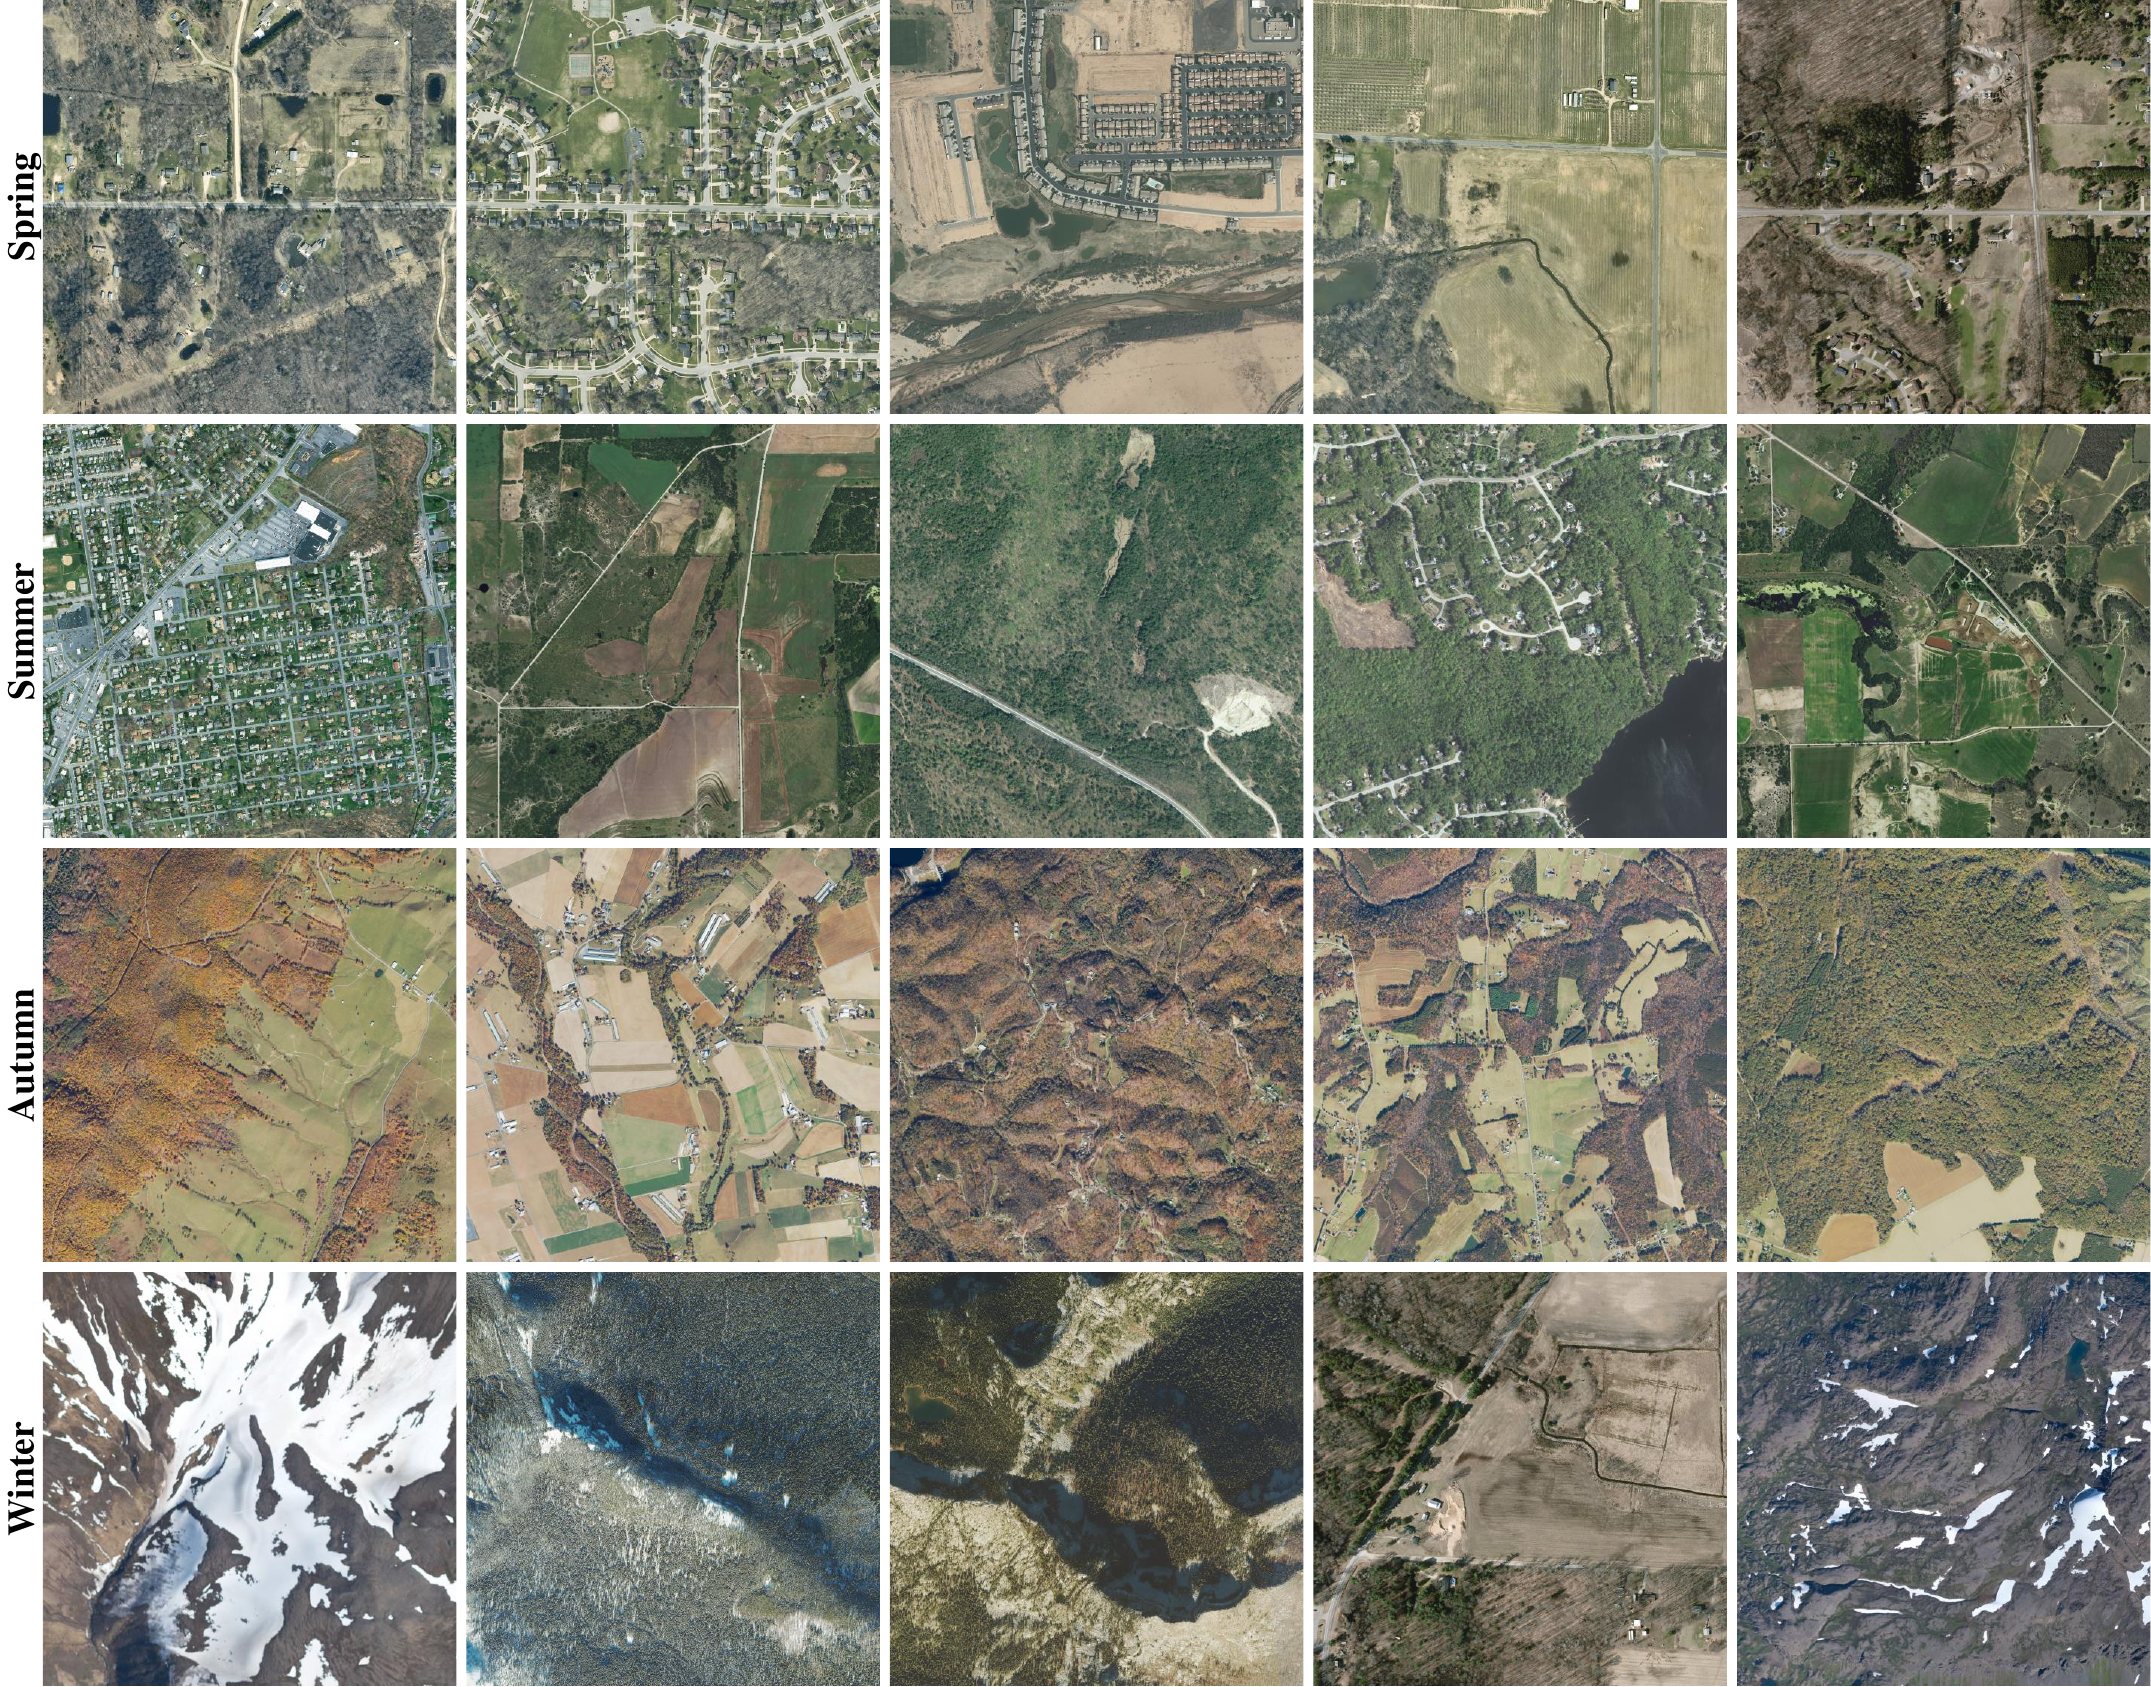}
    \caption{Seasonal Variation in the \emph{8KDehaze} Dataset. Samples can be categorized into 4 seasons: spring, summer, autumn, and winter.}
    \label{fig:season}
\end{figure*}

\vspace{0.3\baselineskip}
\noindent\textbf{Seasonal Variation.} Another key aspect of the \emph{8KDehaze} dataset is its seasonal variation. The dataset includes images captured in all four seasons: spring, summer, autumn, and winter. Figure \ref{fig:season} presents some representative samples from each season. These seasonal differences present unique challenges for dehazing algorithms. For example, models may struggle to differentiate between snow-covered ground and haze, as both can appear similarly gray or white. Additionally, the varying vegetation and atmospheric conditions across seasons require models to adapt to diverse environmental conditions. The inclusion of seasonal variation in the \emph{8KDehaze} dataset is essential for developing robust dehazing algorithms capable of generalizing across different times of the year.

\begin{figure*}
    \centering
    \setlength{\belowcaptionskip}{-7pt}
    \includegraphics[width=\linewidth]{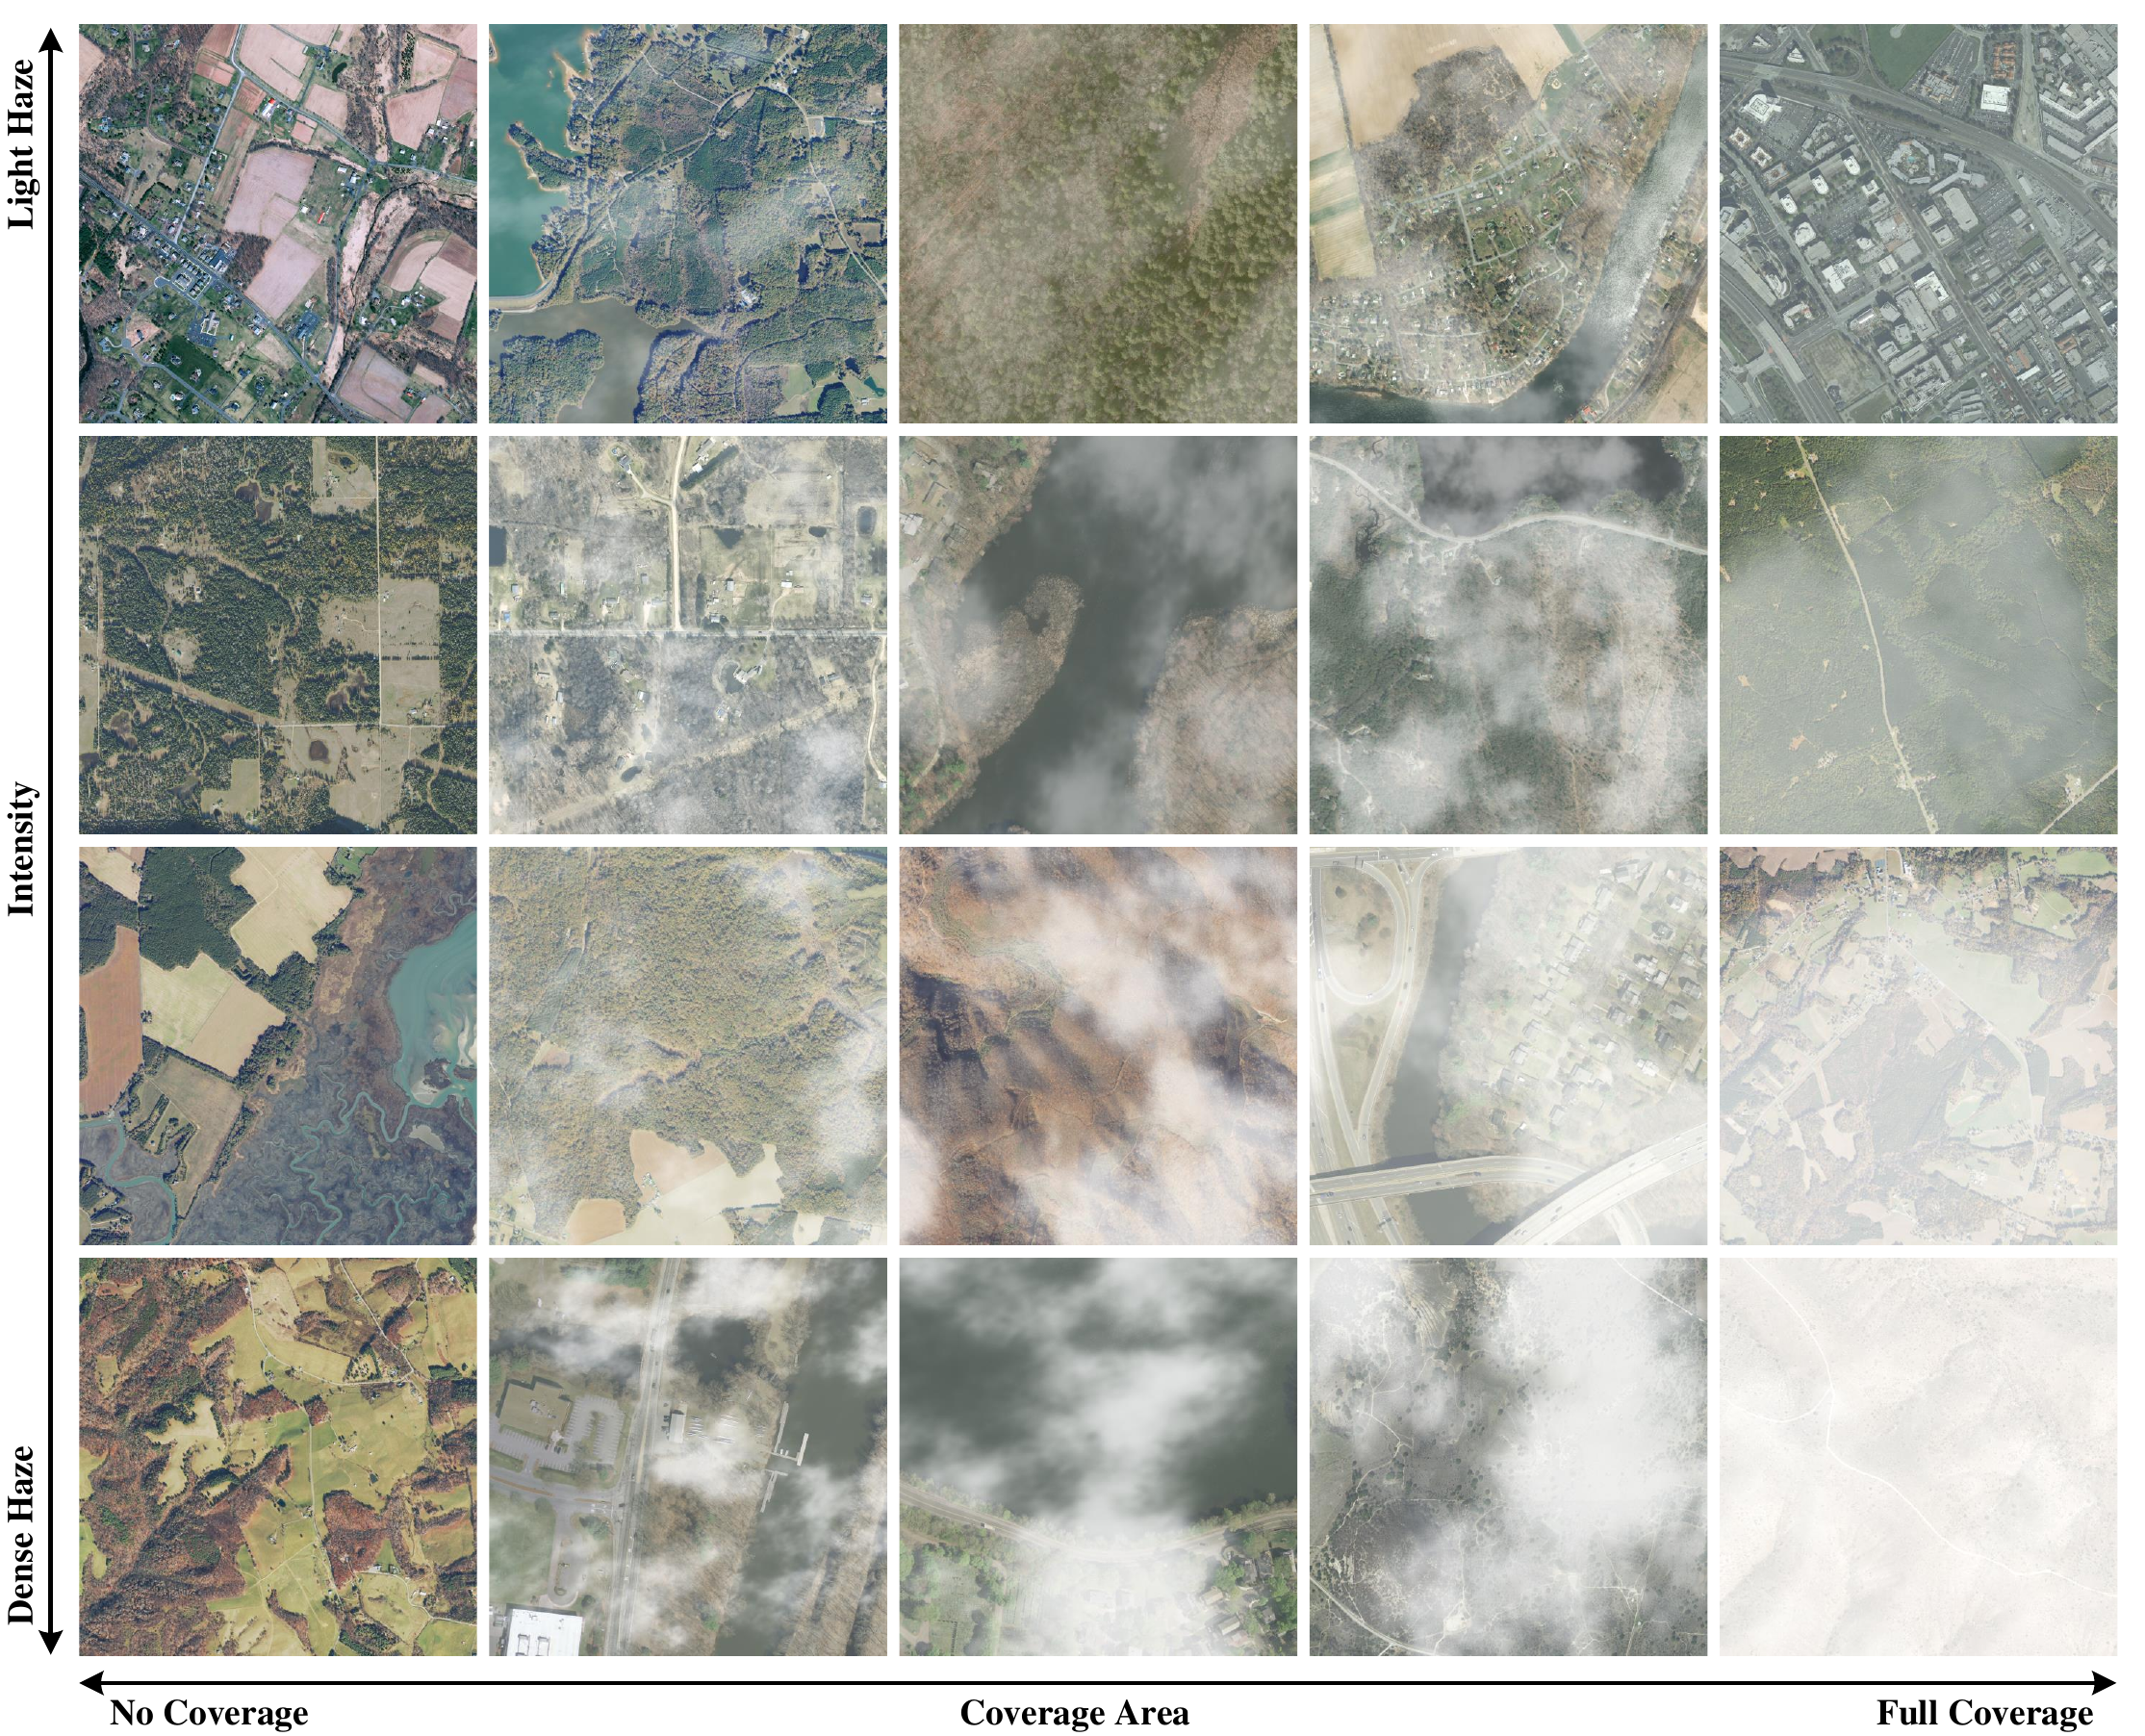}
    \caption{Haze Distribution in the \emph{8KDehaze} Dataset. The x-axis represents the haze coverage area, ranging from no coverage to full coverage, while the y-axis indicates the haze intensity, spanning from low to high.}
    \label{fig:haze}
\end{figure*}

\vspace{0.3\baselineskip}
\noindent\textbf{Haze Distribution.} The \emph{8KDehaze} dataset contains images with diverse haze characteristics. Figure \ref{fig:haze} presents the haze distribution across the dataset, including varying coverage areas and haze intensities. Unlike conventional images captured from a ground-level perspective, aerial images often exhibit irregular and random haze patterns. This non-uniform haze distribution poses significant challenges for dehazing algorithms, as it requires models to effectively utilize global image information and adapt to a wide range of unpredictable haze patterns. Given that most existing dehazing methods primarily address uniform haze in small image patches, the \emph{8KDehaze} dataset's large-sized, non-uniform haze distributions offer new opportunities for advancing the field of image dehazing.

\vspace{0.3\baselineskip}
\noindent\textbf{Dataset Availability.} 
%In accordance with the anonymity requirements of this submission, the complete dataset and access details will be made publicly available in the final published version of this work.
We provide two versions of the dataset: a full version for training and evaluation, and a mini version for debugging. Both the full dataset and the mini version are publicly available at \url{https://github.com/CastleChen339/DehazeXL}.

% Looking ahead, we plan to further enhance the \emph{8KDehaze} dataset’s generalizability and robustness, making it even more valuable for the research community. Our future efforts will include: 1) incorporating additional samples from diverse climatic regions and varying environmental conditions; and 2) improving haze simulation techniques to generate more realistic and varied haze patterns. These enhancements will expand the dataset’s applicability to a wider range of real-world scenarios. 

\vspace{-1mm}
\section{Performance of CNN Backbone Models}
\vspace{-1mm}
As stated in Section Methodology, the proposed DehazeXL uses Swin Transformer~\cite{liu2022swin2} as the backbone for both the Encoder and Decoder. Given the advancements made by CNN-based backbones in the dehazing domain, we conduct additional experiments in this section using several CNN-based backbones for both the Encoder and Decoder. We select the following CNN-based architectures for comparison: VGG-19~\cite{simonyan2014very}, ResNet-50~\cite{he2016deep}, DenseNet-201~\cite{huang2017densely}, and EfficientNet-B4~\cite{tan2019efficientnet}. The models were trained and evaluated on the \emph{8KDehaze}, \emph{4KID}, and \emph{O-HAZE} datasets under the same experimental settings as DehazeXL. The quantitative results are summarized in Table \ref{tab:backbone_8k} to \ref{tab:backbone_ohaze}.

\begin{table}[ht]
\centering
\caption{Performance comparison of different backbones on the \emph{8KDehaze} dataset in terms of PSNR and SSIM}
\setlength{\tabcolsep}{6.5mm}
\fontsize{9}{12}\selectfont{
\begin{tabular}{c|c|c}
\hline
\textbf{Model Backbone}              & \textbf{PSNR}  & \textbf{SSIM} \\ \hline
VGG-19                               & 27.15& 0.9389\\
ResNet-50                            & 28.18          & 0.9583      \\
DenseNet-201                         & 29.49          & 0.9620          \\
EfficientNet-B4                      & 30.15          & 0.9746          \\ 
\textbf{Swin-T (DehazeXL)} & \textbf{32.35} & \textbf{0.9863} \\ \hline
\end{tabular}}
\label{tab:backbone_8k}
\end{table}

\begin{table}[ht]
\centering
\caption{Performance comparison of different backbones on the \emph{4KID} dataset in terms of PSNR and SSIM}
\setlength{\tabcolsep}{6.5mm}
\fontsize{9}{12.5}\selectfont{
\begin{tabular}{c|c|c}
\hline
\textbf{Model Backbone}              & \textbf{PSNR}  & \textbf{SSIM} \\ \hline
VGG-19                               & 23.17& 0.8782\\
ResNet-50                            & 24.20          & 0.8903\\
DenseNet-201                         & 24.81          & 0.8892\\
EfficientNet-B4                      & 25.17          & 0.8946\\ 
\textbf{Swin-T (DehazeXL)} & \textbf{26.62} & \textbf{0.9073} \\ \hline
\end{tabular}}
\label{tab:backbone_4k}
\vspace{-3mm}
\end{table}

\begin{table}[ht]
\centering
\caption{Performance comparison of different backbones on the O-HAZE dataset in terms of PSNR and SSIM}
\setlength{\tabcolsep}{6.5mm}
\fontsize{9}{12}\selectfont{
\begin{tabular}{c|c|c}
\hline
\textbf{Model Backbone}              & \textbf{PSNR}  & \textbf{SSIM} \\ \hline
VGG-19                               & 19.95& 0.7056\\
ResNet-50                            & 20.62          & 0.7184          \\
DenseNet-201                         & 20.88          & 0.7215          \\
EfficientNet-B4                      & 21.06          & 0.7330          \\ 
\textbf{Swin-T (DehazeXL)} & \textbf{21.49} & \textbf{0.7348} \\ \hline
\end{tabular}}
\label{tab:backbone_ohaze}
\vspace{-3mm}
\end{table}

The results indicate that models using CNN-based architectures as both Encoder and Decoder achieve competitive performance in terms of PSNR and SSIM, demonstrating the general applicability of the proposed framework. However, models based on Swin Transformer as the backbone outperform these CNN-based models. This superior performance underscores the advantages of Transformer-based Encoder-Decoder architectures, which are more effective at capturing long-range dependencies compared to traditional CNN architectures. These capabilities make Transformer-based models better suited for image dehazing tasks. Therefore, we choose Swin Transformer as the default encoder and decoder backbone for DehazeXL. Notably, our method achieves state-of-the-art performance without any modifications to the original Swin Transformer, further validating the potential of the proposed framework.

\section{Additional Visual Results}
\vspace{-2mm}
In this section, we present additional visual results to further highlight the effectiveness of the proposed DehazeXL model for large image dehazing. Figure \ref{fig:sup1} illustrates the comparative results of all methods on the \emph{8KDehaze}, \emph{4KID}, and \emph{O-HAZE} datasets. Figure \ref{fig:sup2} showcases the attribution maps for DehazeXL’s dehazed results using the proposed DAM. It offers insight into the specific contributions of each pixel to the dehazed results in the specified region. The source code of DAM is available at \url{https://github.com/fengyanzi/DehazingAttributionMap}.

\begin{figure*}
    \centering
    \includegraphics[width=\linewidth]{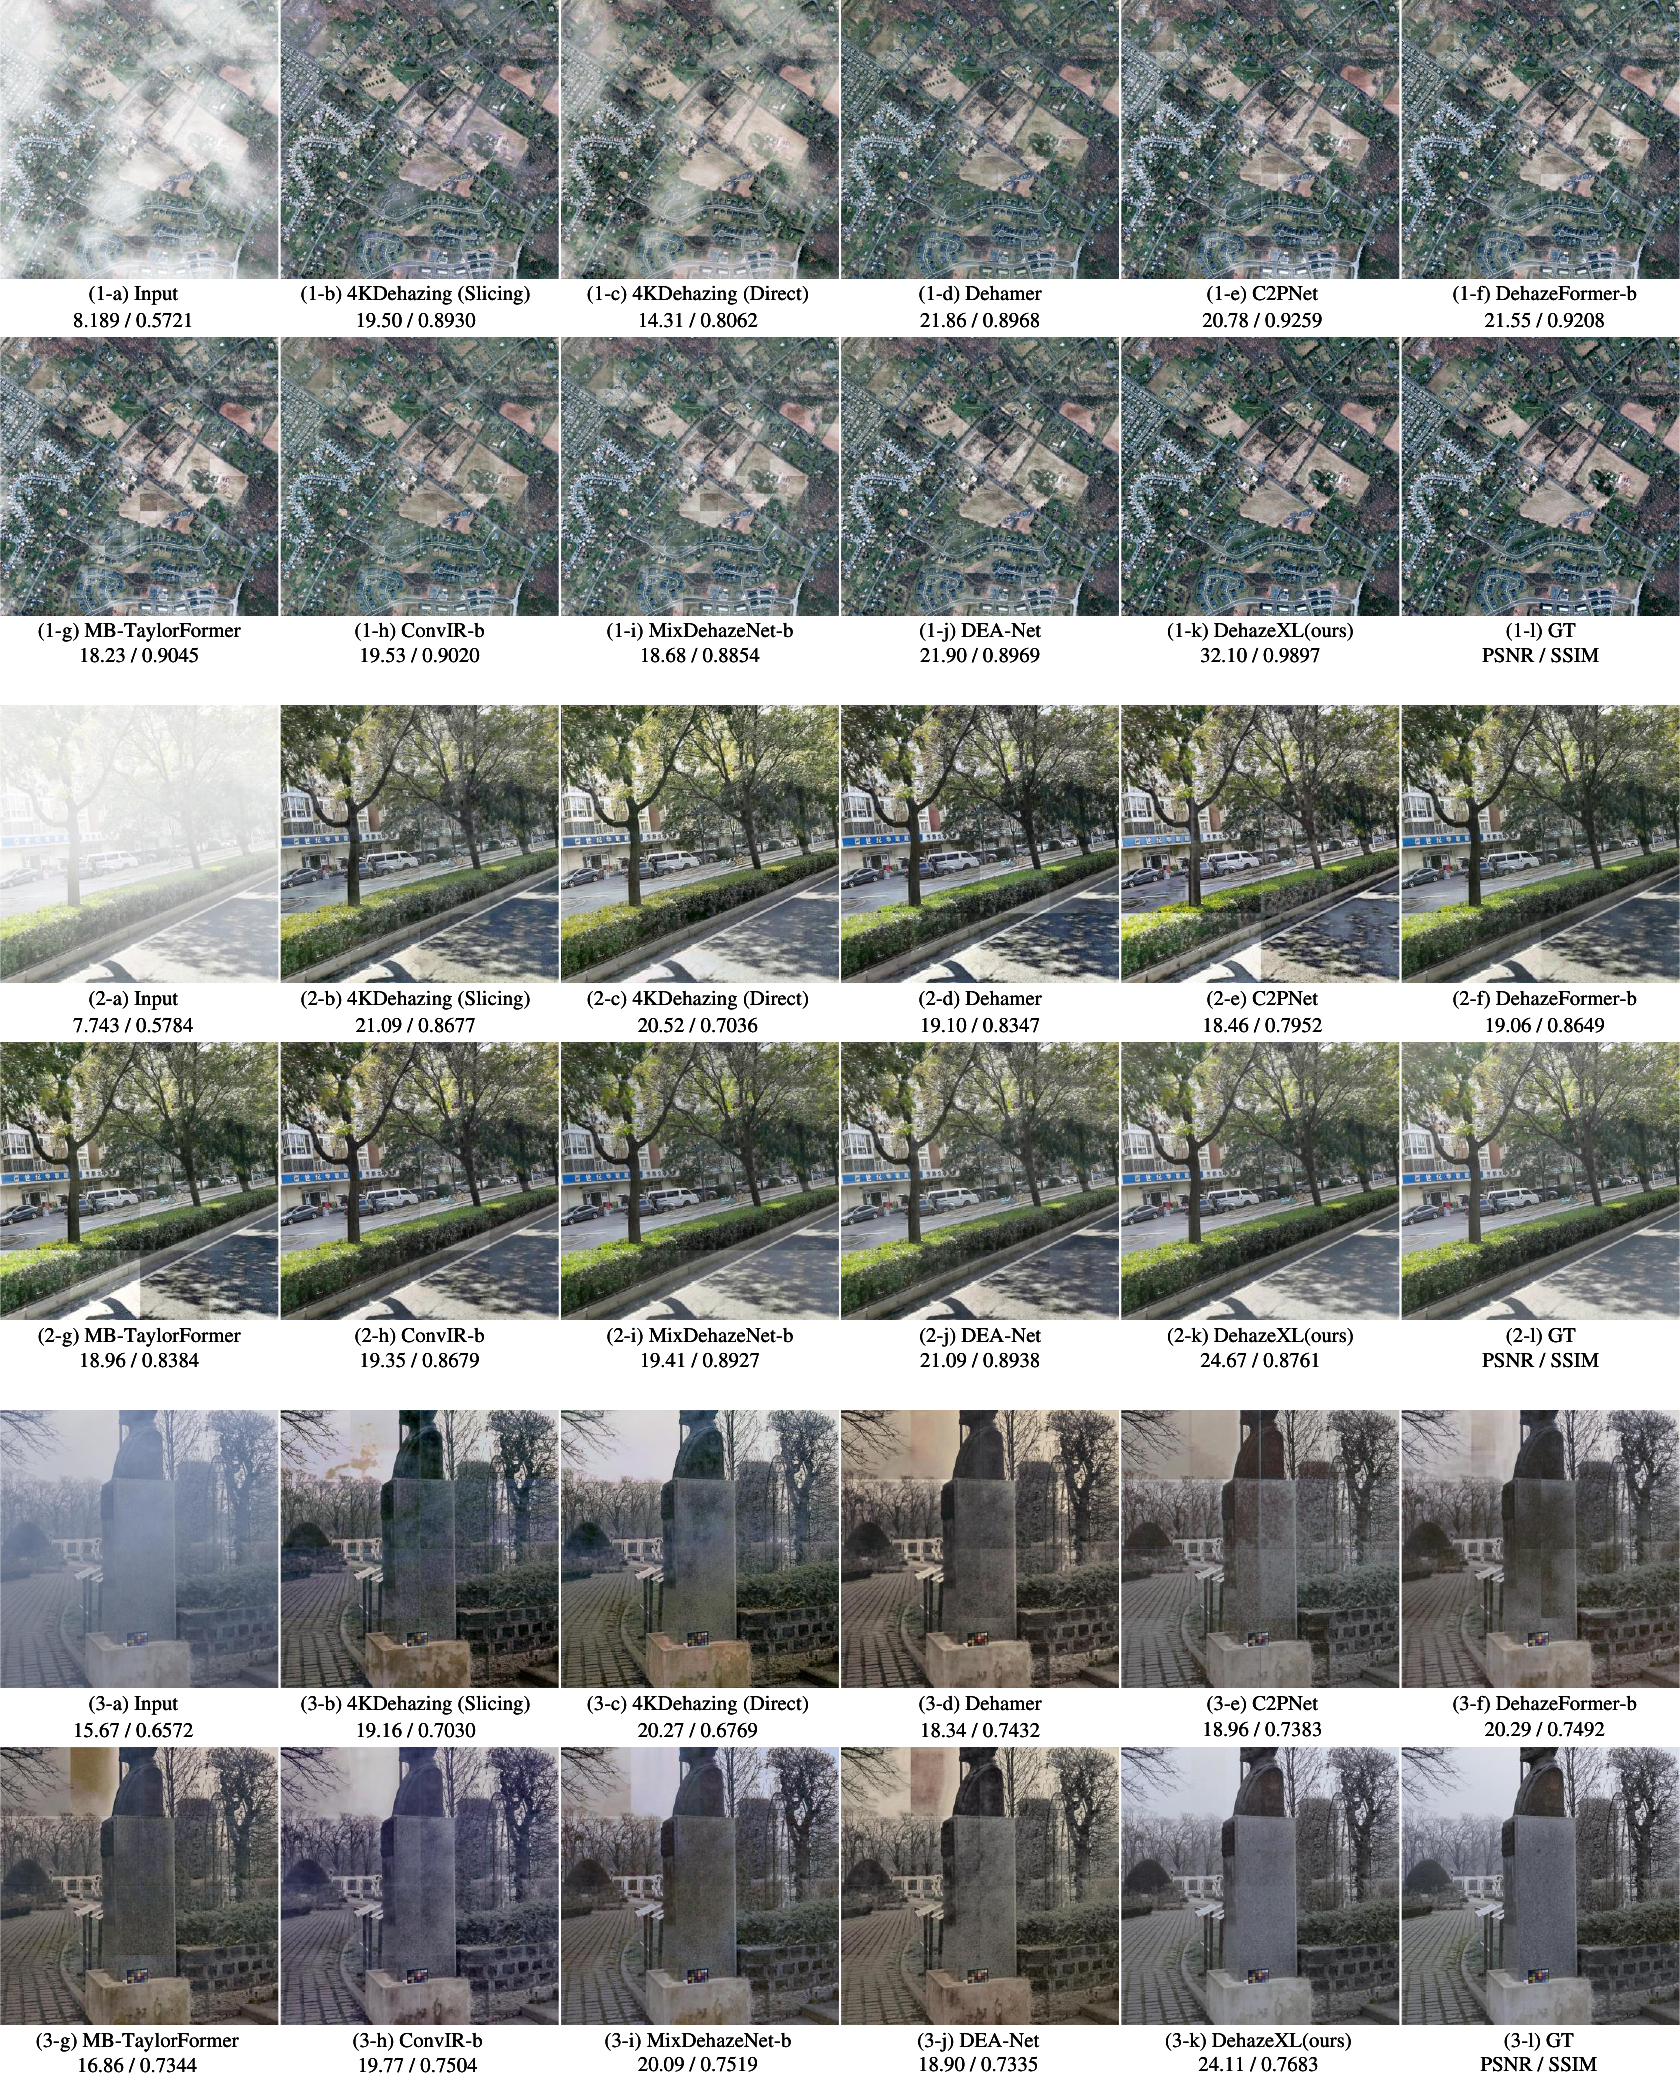}
    \caption{Comparisons of dehazed results on the \emph{8KDehaze}, \emph{4KID}, and \emph{O-HAZE} datasets.}
    \label{fig:sup1}
\end{figure*}

\begin{figure*}
    \centering
    \includegraphics[width=0.91\linewidth]{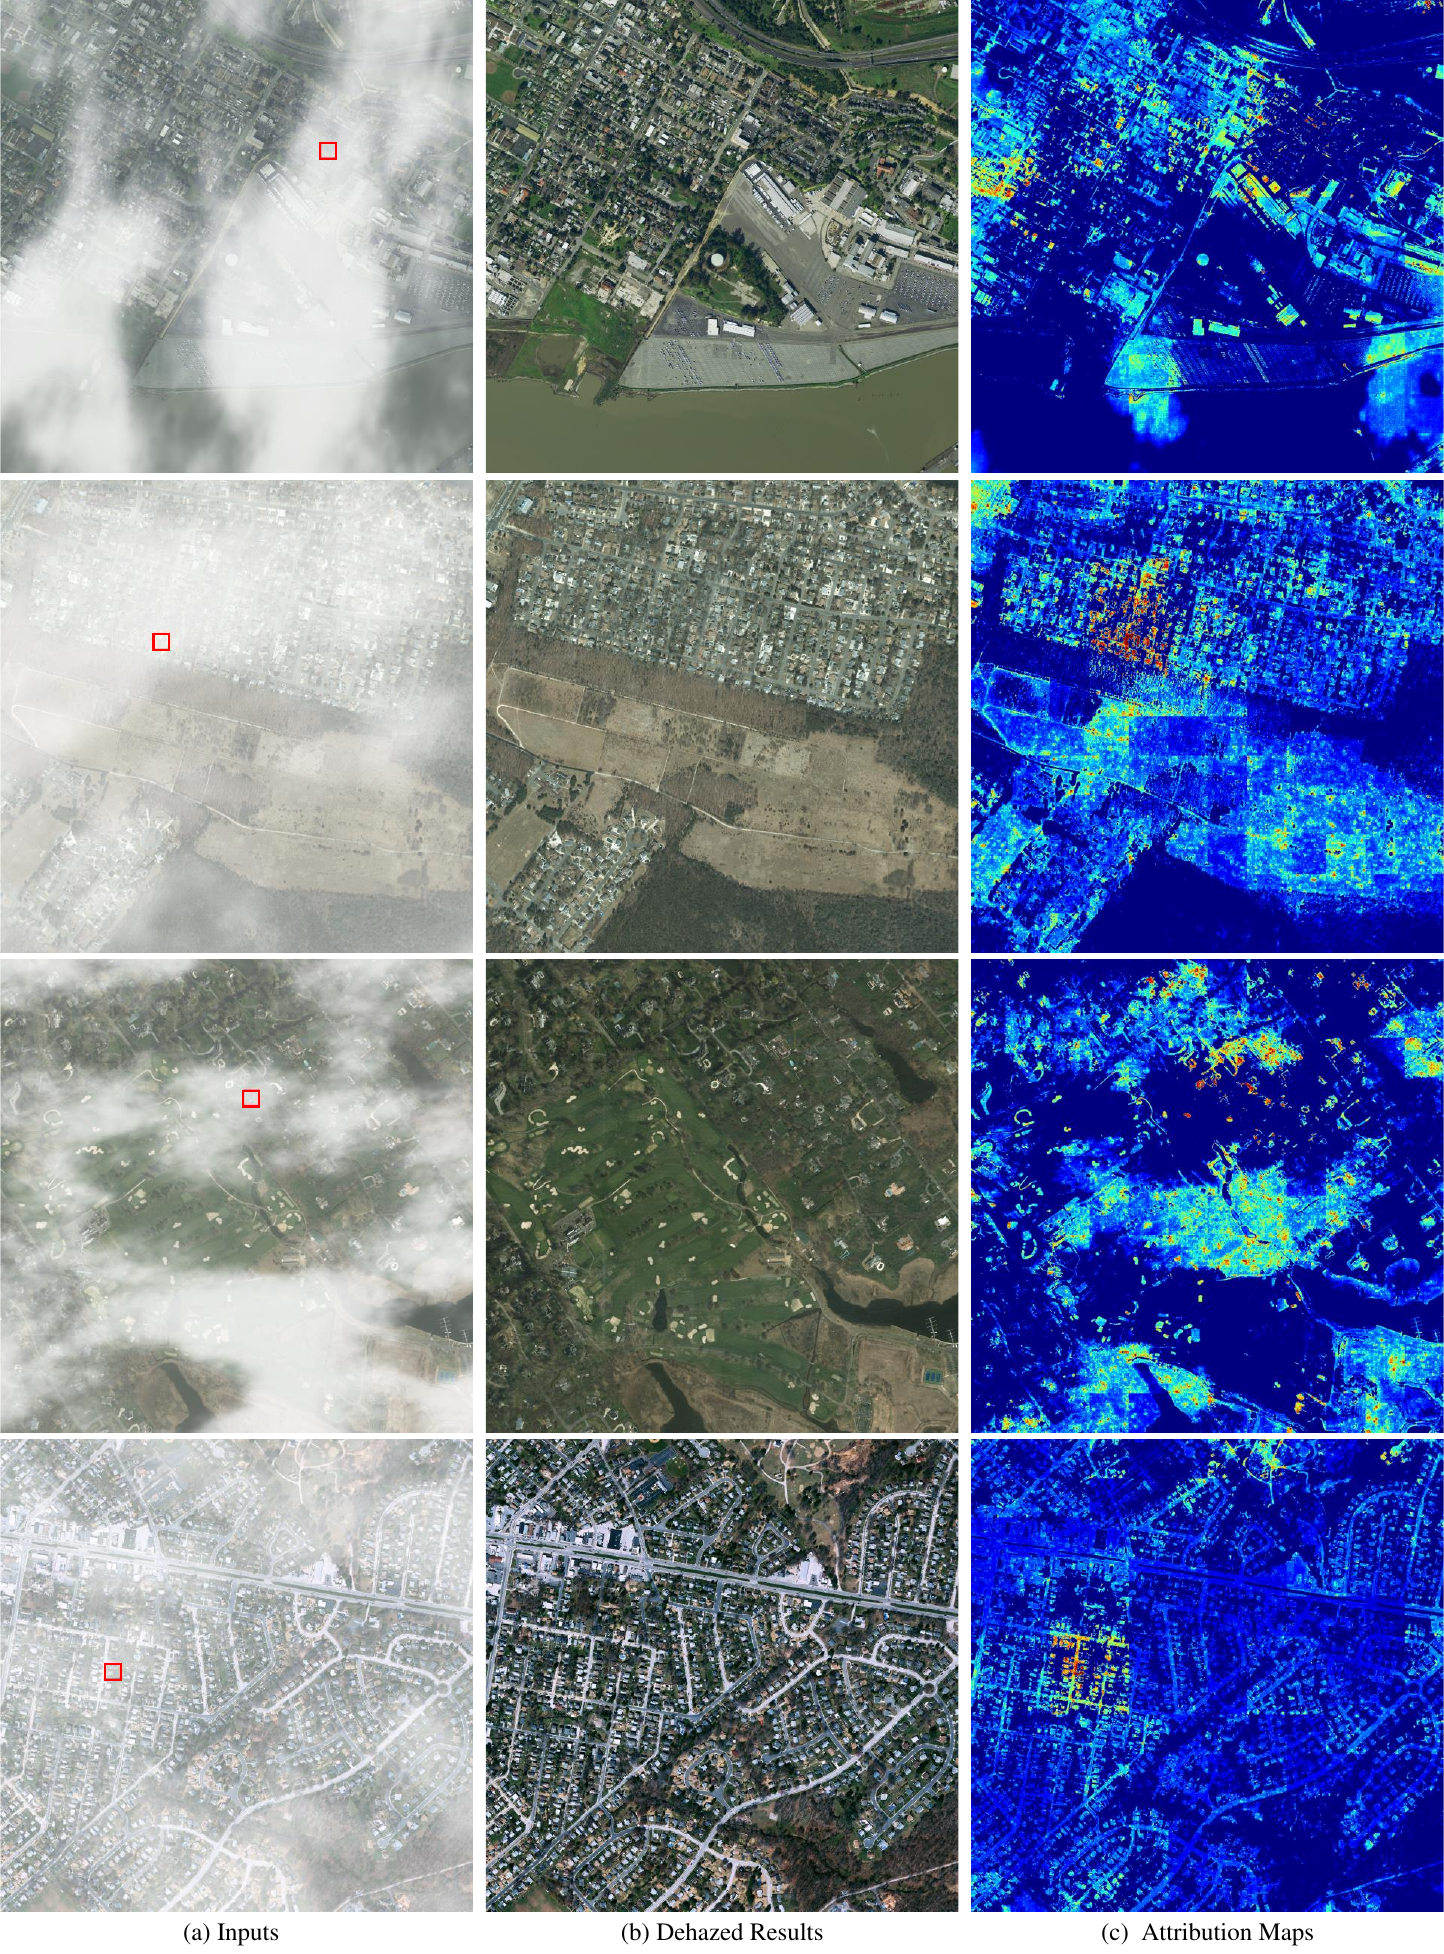}
    \caption{Attribution maps for DehazeXL’s dehazed results using the proposed DAM method. The red box on (a) indicate the regions of interest for attribution. In the attribution maps, the color intensity corresponds to the degree of influence on the dehazed results, with warmer colors (e.g., red) indicating higher influence and cooler colors (e.g., blue) indicating lower influence.}
    \label{fig:sup2}
\end{figure*}
